# Supplementary material for: Berry phase in superconducting multiterminal quantum dots
Source: arXiv:1904.03132 ancillary file (2020-12-13)
Supplement: Supplementary file 1 [file Supplemental_prb_v2.pdf]

# Berry phase in multiterminal superconducting quantum dots: Supplemental Material

Benoît Douçot,<sup>1</sup> Romain Danneau,<sup>2</sup> Kang Yang,<sup>1,3</sup> Jean-Guy Caputo,<sup>4</sup> and Régis Mélin<sup>5</sup>

<sup>1</sup>*Laboratoire de Physique Théorique et Hautes Energies,*

*Sorbonne Université and CNRS UMR 7589, 4 place Jussieu, 75252 Paris Cedex 05, France*

<sup>2</sup>*Institute of Nanotechnology, Karlsruhe Institute of Technology, D-76021 Karlsruhe, Germany*

<sup>3</sup>*Laboratoire de Physique des Solides, CNRS UMR 8502,*

*Univ. Paris-Sud, Université Paris-Saclay F-91405 Orsay Cedex, France*

<sup>4</sup>*Laboratoire de Mathématiques, INSA de Rouen, Avenue de l'Université, F-76801 Saint-Etienne du Rouvray, France*

<sup>5</sup>*Univ. Grenoble-Alpes, CNRS, Grenoble INP, Institut NEEL, 38000 Grenoble, France*

(Dated: December 13, 2020)

The following Supplemental Material contains some of the technical details of the analytical calculations. Section I shows how to treat the reflections induced at gap edges. Section II provides extra numerical results on the resolvent. Section III describes the solution of the transport equation.

## I. REFLECTIONS INDUCED AT GAP EDGES

Now, we consider the regions  $|E + \xi| > \Delta$ , in which the quasiparticle energies are above the BCS gap (see the green lines on Fig. 4 in the article). Physically, periodic driving induces a coupling between Andreev bound states and quasiparticle continua in the leads *via* multiple Andreev reflections. This is manifested in the formalism by the fact that the matrices  $M_0(m)$ ,  $M_{\pm}(m)$  are no longer hermitian [see Eqs. (21) and (22) of the main text]. This abrupt change when  $|E + \xi|$  crosses  $\Delta$  has a quantitatively small, but physically important effect on the energies of the Wannier-Stark ladders. Indeed, the Bohr-Sommerfeld condition (Eq. (B23) in the Appendix of the main text) has been obtained under assumption that we have only exponentially decaying waves at the left of  $\xi_1$  and at the right of  $\xi_4$ . But this simplification did not take into account the nonhermitian dissipative regions at  $|E + \xi| > \Delta$ . To take them into account, we have to consider that a decaying wavefunction in the interval  $\xi_4 < \xi < \xi_{\Delta} = -E + \Delta$  will undergo reflection at the interface located at  $\xi_{\Delta}$ , which will subsequently modify the matching condition at the turning point located at  $\xi_4$ . The same reasoning holds for the turning point located at  $\xi_1$ . This will introduce exponentially small corrections in the Bohr-Sommerfeld condition, which will push the energies of the Wannier-Stark ladder levels slightly below the real axis.

In principle, we could try to obtain the matching conditions of semiclassical solutions at the gap crossing within a semiclassical analysis. Indeed, near  $\xi_{\Delta}$ ,  $k(\xi)$  is complex and from Eq. (27) in the main text,  $k(\xi) - k(\xi_{\Delta})$  is proportional to  $(\xi - \xi_{\Delta})^{1/2}$ . We have seen in subsection IV.B in the main text that  $k(\xi_{\Delta})$  is complex when  $\varphi_q \neq 0 \bmod 2\pi$ , and thus  $\Im k(\xi_{\Delta}) \neq 0$ . One can then show that the WKB Ansatz remains valid as long as  $\varepsilon \frac{k'(\xi)}{(\Im k(\xi_{\Delta}))^2} \ll 1$ . Since  $k'(\xi)$  diverges as  $|\xi - \xi_{\Delta}|^{-1/2}$ , the previous criterion holds until  $\xi$  becomes very close to  $\xi_{\Delta}$ , up to  $O(\varepsilon^2)$ . Since  $\xi = 2m\omega_0$ , the WKB Ansatz applied to the discrete Eq. (15) is expected to remain very accurate everywhere, except for the two integers  $m$  such

that  $|2m\omega_0 - \Delta| < 2\omega_0$ . Solving explicitly Eq. (15) for these two values of  $m$  can thus provide the wanted reflection matrix for the two evanescent waves incoming at  $\xi_{\Delta}$  from below. We do not proceed further along this line however, because for the sake of actually computing the resolvent, it is easier and faster to do it numerically, than from semiclassical expressions. Indeed, the latter involve various integrals taken around various cycles of the classical trajectory, for which closed analytical expressions are not available.

## II. SUPPLEMENTAL NUMERICAL RESULTS ON THE RESOLVENT

In this section of the Supplemental Material, we further validate numerically some of the predictions of the semiclassical approximation at small voltage, such that  $eV/\Delta \ll 1$ . The support of the resolvent  $\mathcal{R}(E) = [E - \mathcal{H}]^{-1}$  is indeed expected to be mostly located on the projection of the classical trajectories  $\mathcal{T}_{E,\sigma}$  along the  $\xi$  axis. This expectation is well confirmed by the following direct numerical computation of the resolvent, as shown on Fig. 1 in this Supplemental Material. For the parameters chosen there, the two Wannier-Stark ladders are far from degenerate, and this manifests itself by the fact that one ladder (red on Fig. 1) lives mostly in the upper Andreev band, while the other ladder (blue on Fig. 1) is concentrated on the lower Andreev band.

It is interesting to look in more detail at the behavior of the resolvent for nearly degenerate Wannier-Stark ladders. There, we expect that Landau Zener tunneling will superpose these two contributions to the resolvent. This is clearly seen on Fig. 2 (c), and on Fig. 3 (c)-(d). The main difference between Fig. 2 and Fig. 3 is that level repulsion is much stronger in the latter than in the former. This explains why it is possible to see on Fig. 2 the cross-over from a resolvent localized on a single band to the mixed configuration of panel (c).

## III. SOLUTION OF THE TRANSPORT EQUATION

Let us start with Eq. (A23) in the Appendix of the main text. We assume to have chosen a smooth frame  $|e(\xi, k(\xi))\rangle$ , such that  $L_0(\xi, k(\xi))|e(\xi, k(\xi))\rangle = 0$ . We write  $|\chi_0(\xi)\rangle = f(\xi)|e(\xi, k(\xi))\rangle$ , where the function  $f(\xi)$  satisfies the first

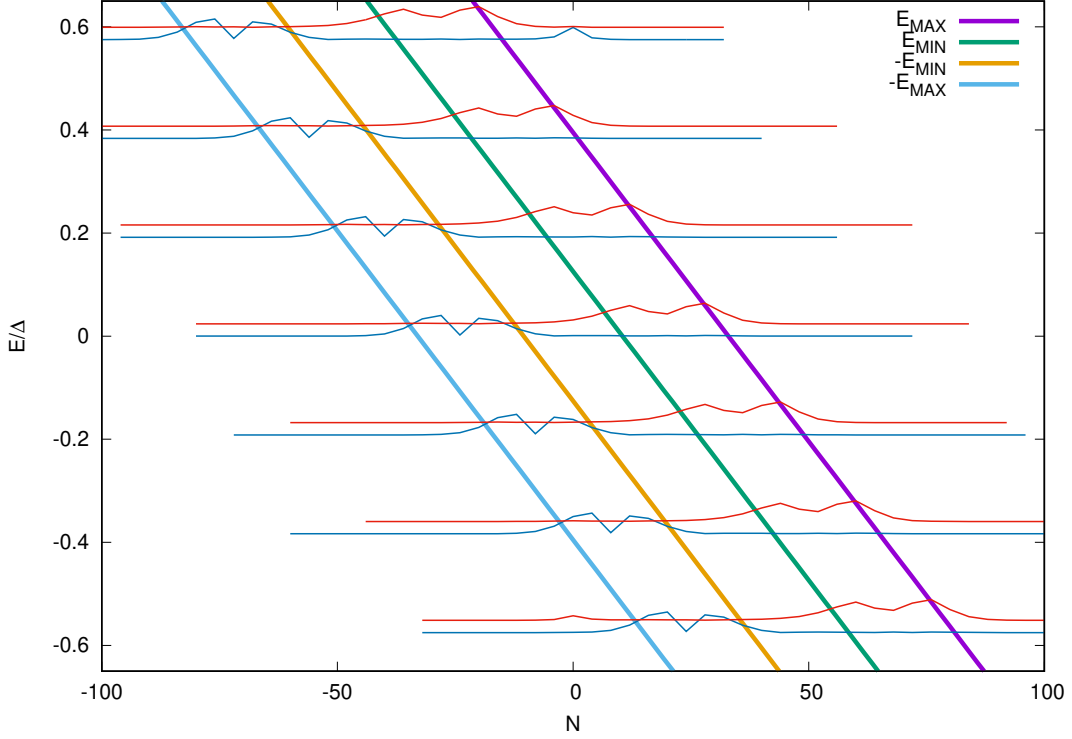

FIG. 1. *Tilted band picture seen in the resolvent*: plots of  $\mathcal{R}(E)_{N,w;0,v}$ , as a function of  $N$  for various values of  $E$ , all corresponding to Wannier-Stark resonances. The parameters are:  $\Delta/eV = 83.45$ ,  $\Gamma_a/\Delta = 0.4$ ,  $\Gamma_b/\Delta = 0.2$ ,  $\Gamma_c/\Delta = 0$ , and  $\varphi_q/2\pi = 0$ . The figure shows the resolvent in the electron-electron channel. The projection of the classical trajectory  $\mathcal{T}_{E,+}$  (resp.  $\mathcal{T}_{E,-}$ ) along the  $\xi$  axis corresponds to the interval  $[E_{MIN}, E_{MAX}]$  (resp.  $[-E_{MAX}, -E_{MIN}]$ ). Recall that we have defined  $\xi = N\omega_0$ .

order differential equation:

$$2\langle e|K|e\rangle\frac{df}{d\xi} + \left(2\langle e|K|\frac{de}{d\xi}\rangle + \langle e|\frac{dK}{d\xi}|e\rangle\right)f = 0. \quad (1)$$

Suppose that, for a choice of local right and left eigenvectors, we have:

$$\langle e|K|\frac{de}{d\xi}\rangle = \langle \frac{de}{d\xi}|K|e\rangle. \quad (2)$$

Then, Eq. (1) becomes equivalent to:

$$\frac{d}{d\xi} \left( \langle e|K|e\rangle^{1/2} f \right) = 0. \quad (3)$$

The condition (2) is now reformulated in a simpler way. Taking the total derivative with respect to  $\xi$  of  $L_0(\xi, k(\xi))|e(\xi, k(\xi))\rangle = 0$ , and using Eq. (A22) of the Appendix in the main text, we get

$$((1+c)I + 2k'(\xi)K)|e\rangle + L_0|\frac{de}{d\xi}\rangle = 0 \quad (4)$$

Multiplying on the left by  $\langle e|$  leads to the following useful relation:

$$(1+c)\langle e|e\rangle + 2k'(\xi)\langle e|K|e\rangle = 0. \quad (5)$$

Similarly, we obtain

$$\langle e|((1+c)I + 2k'(\xi)K)) + \langle \frac{de}{d\xi}|L_0 = 0. \quad (6)$$

Multiplying Eq. (4) on the left by  $\langle \frac{de}{d\xi}|$ , and Eq. (6) on the right by  $|\frac{de}{d\xi}\rangle$ , subtracting the results, and applying Eq. (5) leads to

$$\frac{\langle e|K|\frac{de}{d\xi}\rangle - \langle \frac{de}{d\xi}|K|e\rangle}{\langle e|K|e\rangle} = \frac{\langle e|\frac{de}{d\xi}\rangle - \langle \frac{de}{d\xi}|e\rangle}{\langle e|e\rangle}. \quad (7)$$

To proceed further, we have to make explicit choices of frames. With the approximate forms of  $M_0$  and  $M_{\pm}$  matrices given in Eqs. (A17) to (A19) of the Appendix in the main text, the  $L_0$  operator takes the form:

$$L_0(\xi, k) = \begin{pmatrix} \sigma(\rho(k)\rho(k^*))^{1/2} & -\rho(k)e^{i\alpha(k)} \\ -\rho(k^*)e^{-i\alpha(k)} & \sigma(\rho(k)\rho(k^*))^{1/2} \end{pmatrix}, \quad (8)$$

where  $\rho(k)$  and  $\rho(k^*)$  are non negative real numbers, which are equal when  $k$  is real;  $\alpha(k)$  is also a real number and  $\sigma = \pm 1$  is the sign of  $E + \xi$ . We choose the right and left

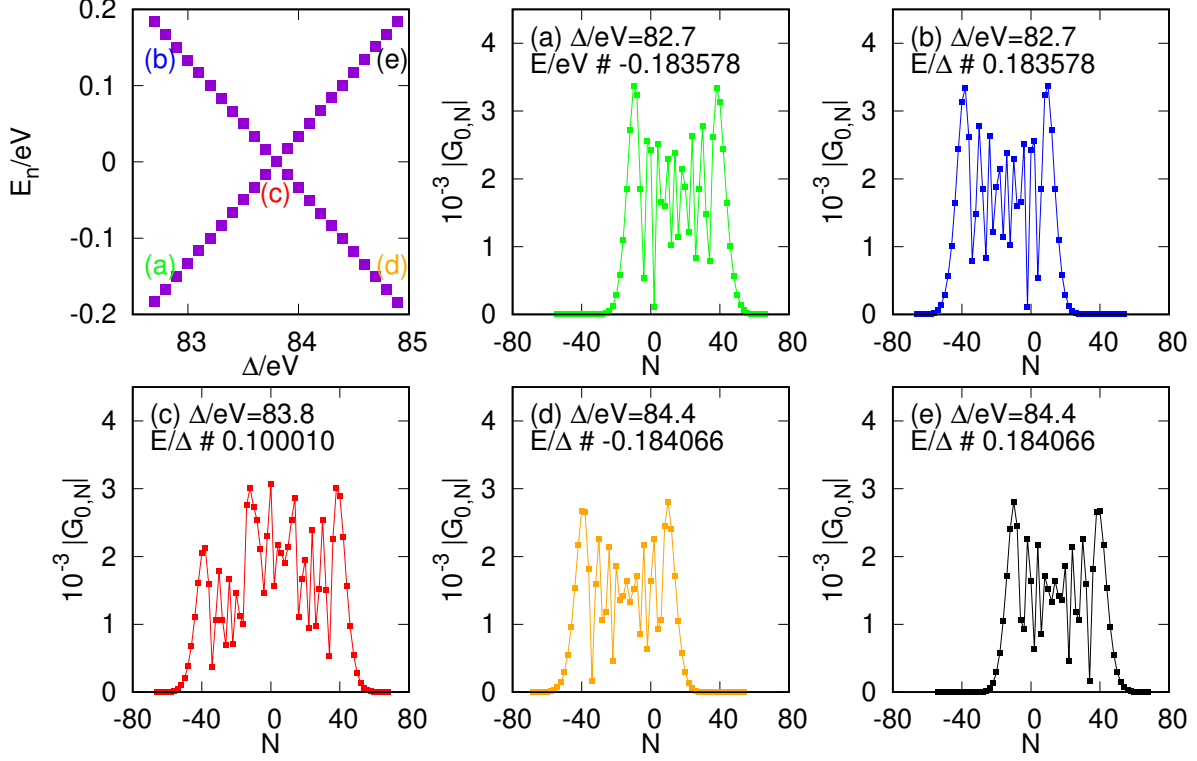

FIG. 2. *Resolvent close to an avoided crossing*: The top left panel is a zoom of the spectrum for the following parameters:  $\Gamma_a/\Delta = 0.4$ ,  $\Gamma_b/\Delta = 0.2$ ,  $\Gamma_c/\Delta = 0$ ,  $\phi_q/2\pi = 0$ . The panels (a)-(e) correspond to different choices of voltages and energies for which the resolvent  $|\mathcal{R}(E)_{N,w;0,v}|$  is plotted as a function of  $N$ .

eigenvector frames according to:

With these choices, we have  $\langle e|e \rangle = 2$ , and Eq. (5) implies

$$\langle e|K|e \rangle = -\frac{1+c}{k'(\xi)}. \quad (9)$$

We also have

$$\langle e|\frac{de}{d\xi}\rangle = \langle \frac{de}{d\xi}|e \rangle = 0. \quad (10)$$

It is deduced from Eq. (7), that the condition given by Eq. (2) is satisfied. This implies that Eq. (3) holds. Using Eq. (9), we obtain

$$f(\xi) = \text{cte } k'(\xi)^{1/2}. \quad (11)$$

$$|e\rangle = \left( \sigma \left( \frac{\rho(k)}{\rho(k^*)} \right)^{1/4} e^{i\frac{\alpha(k)}{2}}, \left( \frac{\rho(k^*)}{\rho(k)} \right)^{1/4} e^{-i\frac{\alpha(k)}{2}} \right)^T$$

$$\langle e| = \left( \sigma \left( \frac{\rho(k^*)}{\rho(k)} \right)^{1/4} e^{-i\frac{\alpha(k)}{2}}, \left( \frac{\rho(k)}{\rho(k^*)} \right)^{1/4} e^{i\frac{\alpha(k)}{2}} \right).$$

<sup>1</sup> R. Mélin, R. Danneau, K. Yang, J.-G. Caputo, and B. Douçot, *Engineering the Floquet spectrum in superconducting multiterminal quantum dots*, Phys. Rev. B **100**, 035450 (2019).

<sup>2</sup> L. D. Landau, E. M. Lifshitz, *Quantum Mechanics*, Third Ed.,

Butterworth-Heinemann (2008).

<sup>3</sup> R. Mélin, J.-G. Caputo, K. Yang, J.-G. Caputo, and B. Douçot, *Simple Floquet-Wannier-Stark-Andreev viewpoint and emergence of low-energy scales in a voltage-biased three-terminal Josephson junction*, Phys. Rev. B **95**, 085415 (2017).

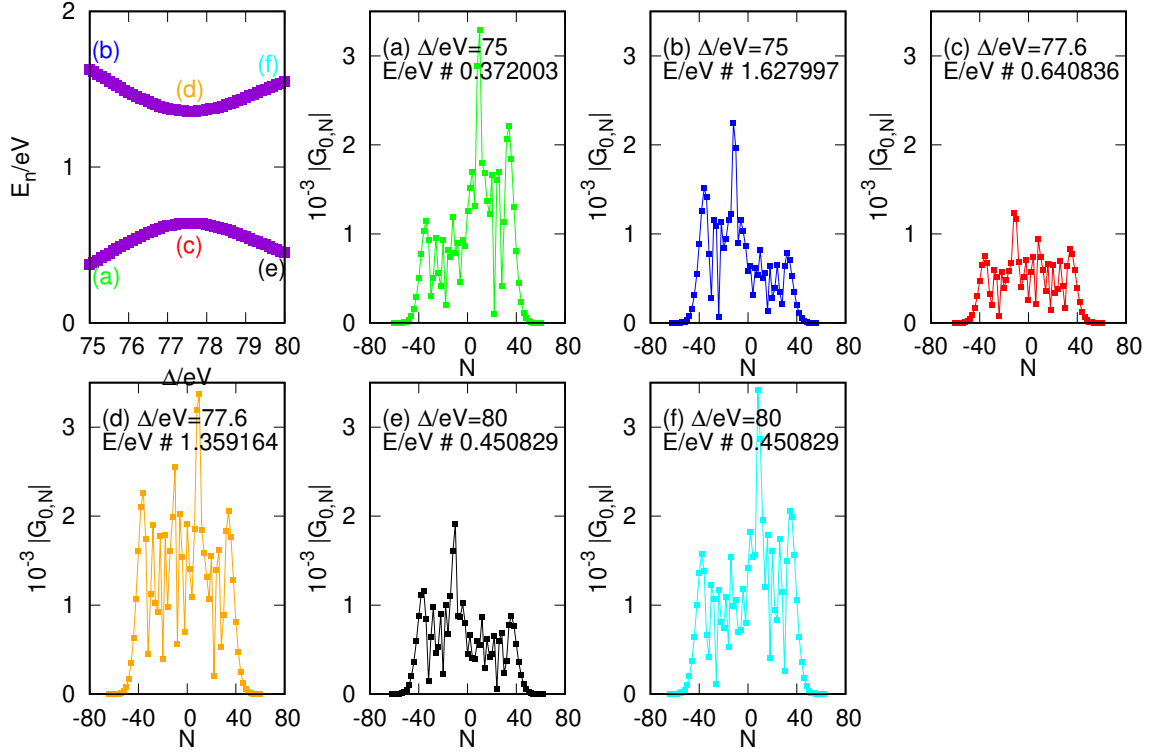

FIG. 3. *Resolvent with large interladder tunneling*: The top left panel is zoom of the spectrum for the following parameters:  $\Gamma_a/\Delta = \Gamma_b/\Delta = \Gamma_c/\Delta = 0.3$ ,  $\varphi_q/2\pi = 0.1$ . The labels (a)-(e) correspond to different choices of voltages and energies for which the resolvent  $|\mathcal{R}(E)_{N,w;0,v}|$  is plotted as a function of  $N$ .
